# Supplementary material for: Sirius: Visualization of Mixed Features as a Mutual Information Network Graph
Source: arXiv:2106.05260 source file (2022-08-13)
Supplement: Supplementary file 1 [file appendix.tex]

\section{Appendix}
